# Supplementary material for: Zero-P-to-3: Zero-Shot Partial-View Images to 3D Object
Source: arXiv:2505.23054 source file (2025-05-29)
Supplement: Supplementary file 1 [file X_suppl.tex]

\clearpage
\setcounter{page}{1}
\twocolumn [ %
{\renewcommand\twocolumn[1][]{#1}%
\maketitlesupplementary
\begin{center}
    \centering
    \vspace{-15}
\includegraphics[width=0.95\linewidth]{figures/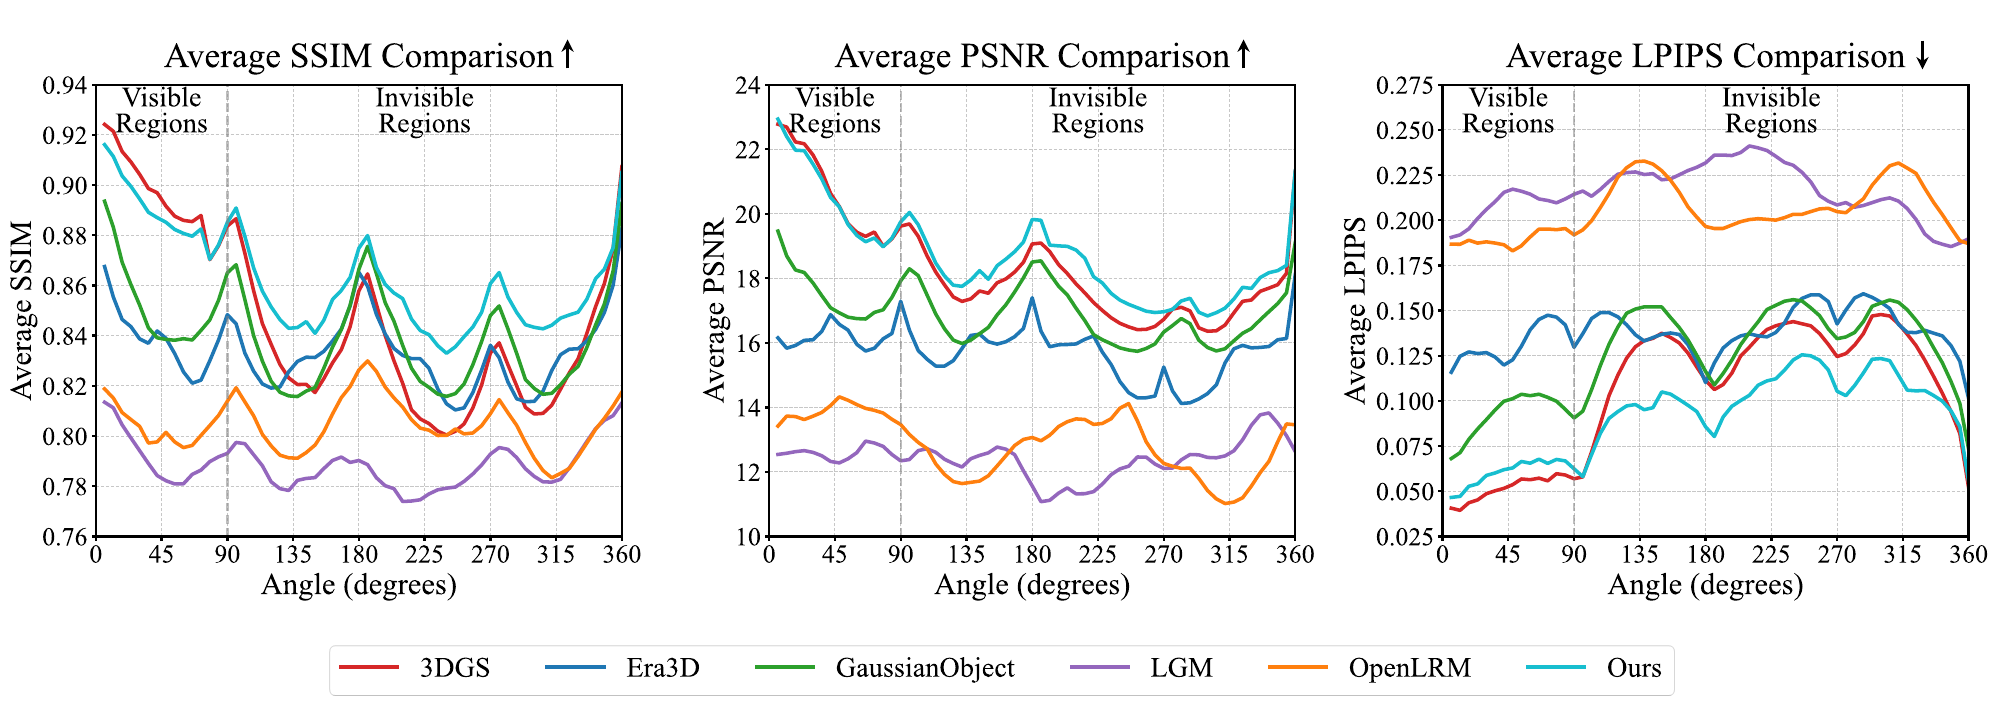}
\captionof{figure}{Comprehensive quantitative analysis across different views. The subplots illustrate the average performance metrics (SSIM, PSNR, and LPIPS) as a function of viewing angle, with visible regions spanning 0-90 degrees and invisible regions covering 90-360 degrees. This visualization enables direct comparison of reconstruction quality between visible and invisible views.}
\label{fig:quan}
\vspace{-5}
\end{center}}
]
\section{More Quantitative Comparison Results}
The quantitative results in Fig.~\ref{fig:quan} demonstrate that our~\method~achieves superior performance across the majority of the evaluation metrics. Notably, while 3DGS~\cite{kerbl20233d} exhibits optimal performance in visible regions, this can be attributed to its training objective being solely focused on matching ground truth in visible regions, potentially leading to overfitting in these regions. More significantly, our~\method~ consistently outperforms the baseline approaches across all invisible regions, demonstrating its robust generalization to novel views.
\section{More Implementation Details}
\subsection{Data Preparation}
Our experimental evaluation employs both synthetic and real-world datasets. The synthetic dataset comprises rendered images from Objaverse~\cite{objaverseXL} and curated 3D models, while our real-world dataset incorporates images from RefNeRF~\cite{verbin2022ref} and custom-captured photographs. For synthetic data generation, we utilize Blender~\footnote{Blender v4.2, https://www.blender.org/} to render images from three elevation angles, with each viewpoint encompassing approximately 90-degree visible regions. The real-world dataset consists of two components: (1) selected images from the RefNeRF dataset with approximately 90-degree visible regions at varying elevations, and (2) approximately 100 frames extracted from video sequences captured using an iPhone 14 Pro, where each sequence was recorded at three distinct elevations with 90-degree coverage around the target object.

\subsection{Pose Estimation}
For the synthetic dataset, we leverage the ground truth camera poses from the rendering process and employ COLMAP for feature extraction, matching, and initial point cloud triangulation. The real-world dataset requires a more comprehensive approach. We first apply the Segment Anything Model (SAM)~\cite{kirillov2023segment} for background removal, followed by COLMAP's complete sparse reconstruction pipeline to obtain initial point clouds and camera poses. 

\subsection{Multi-View Diffusion Framework}
Our implementation utilizes three input views separated by 45 degrees for both qualitative and quantitative evaluations. As illustrated in Fig.~\ref{rotation_supp}, each input (Input n) represents an independent MVD inference process. The framework operates in two primary stages: (1) independent noise prediction via U-Net for each view, and (2) information fusion through weighted averaging during the DDIM sampling process. We employ the Era3D~\cite{li2024era3d} backbone, which is specifically designed to predict five cardinal viewpoints: left-front, left, back, right, and right-back. For viewpoints not directly predicted by Era3D (e.g., Input 1's view 4), our system compensates by leveraging predictions from complementary inputs (e.g., Input 2's view 3 and Input 3's view 5), ensuring comprehensive coverage of the object's geometry. For both Era3D's~\cite{li2024era3d} multi-view diffusion and DiffBIR's~\cite{lin2023diffbir} image denoising diffusion, we employ 50 inference steps to generate supervision images at 512×512 resolution.
\begin{figure}
    \centering
    \includegraphics[width=0.9\linewidth]{figures/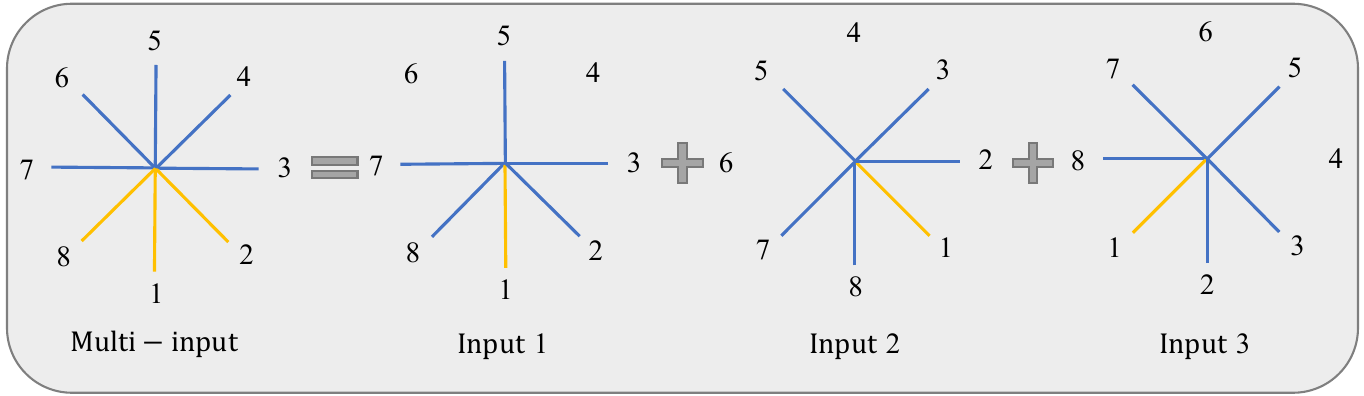}
    \caption{Illustration of three inputs with 45-degree intervals, where yellow lines indicate conditioning views and blue lines represent predicted views.}
    \label{rotation_supp}
    \vspace{-5}
\end{figure}
\begin{figure}
    \centering
    \includegraphics[width=0.612\linewidth]{figures/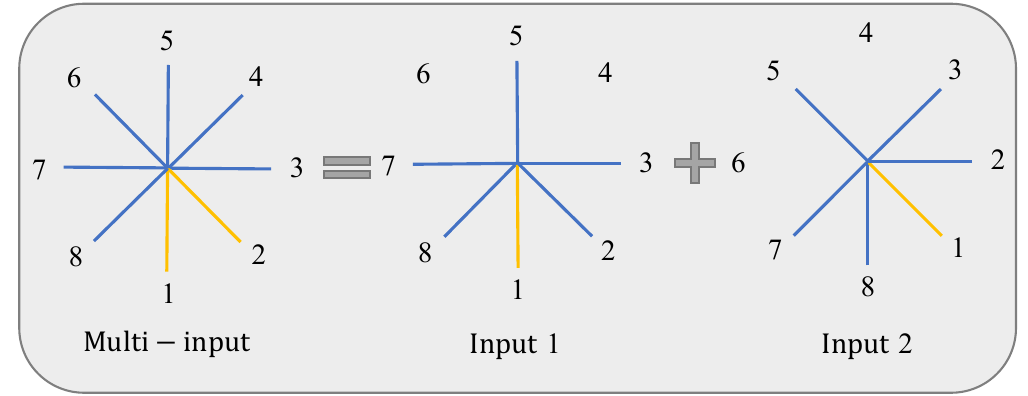}
    \caption{Illustration of two inputs with 45-degree intervals, where yellow lines indicate conditioning views and blue lines represent predicted views.}
    \label{rotation_supp_2}
    \vspace{-5}
\end{figure}
\subsection{Variance Compensation}
The DDIM sampling process with added noise can be decomposed into deterministic and stochastic components:
$$x_{t-1} = \underbrace{\mu_t(x_t, \epsilon_\theta)}_{\text{deterministic}} + \underbrace{\sigma_t\epsilon}_{\text{stochastic}},$$
where $\epsilon \sim \mathcal{N}(0,I)$. In our multi-view setting, the weighted averaging of predictions affects the variance of the deterministic component $\mu_t$. To prevent potential out-of-distribution (OOD) issues, we propose a variance compensation mechanism that maintains the statistical properties of the generated samples.

For each channel $c$, we compute a scaling factor $\lambda_c$ for the stochastic component:
$$\lambda_c = \sqrt{\frac{\text{Var}(x_{t-1}^{\text{orig}}) - \text{Var}(x_{t-1}^{\text{avg}}) + \text{Var}(\sigma_t\epsilon)}{\text{Var}(\sigma_t\epsilon) + \delta}},$$
where $x_{t-1}^{\text{orig}}$ and $x_{t-1}^{\text{avg}}$ represent the original and averaged samples respectively, $\sigma_t\epsilon$ is the stochastic noise term, and $\delta$ is a small constant for numerical stability.
The modified DDIM sampling equation with variance compensation becomes:
$$x_{t-1} = \mu_t(x_t, \epsilon_\theta) + \lambda_c\sigma_t\epsilon.$$
This compensation mechanism ensures that our multi-MVD fusion inference maintains proper statistical properties while benefiting from the information aggregation across multiple views.
\begin{figure}
    \centering
    \includegraphics[width=0.8\linewidth]{figures/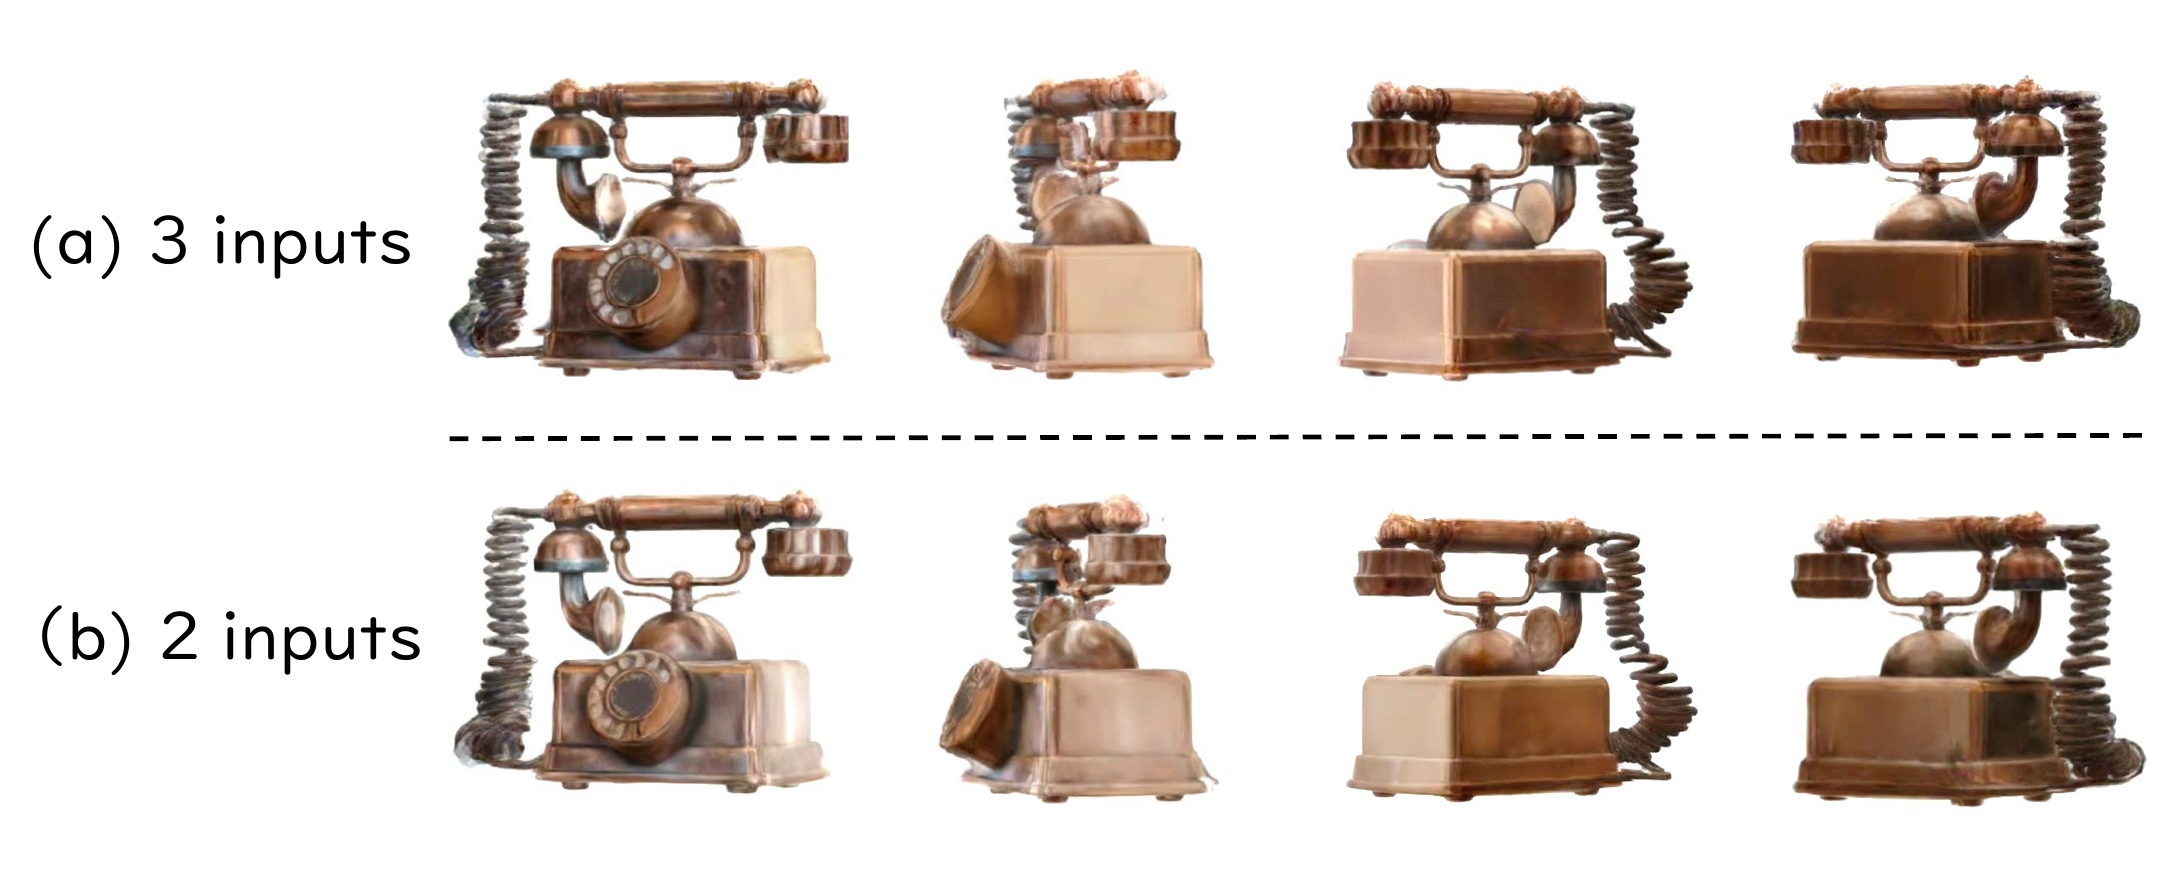}
    \caption{Extension of our \method~ to 3DGS refinement with two 45-degree-separated input views. While the quality shows slight degradation compared to the standard three-input configuration, the refinement results remain satisfactory.}
    \label{45degree}
    \vspace{-5}
\end{figure}
\begin{figure}
    \centering
    \includegraphics[width=0.9\linewidth]{figures/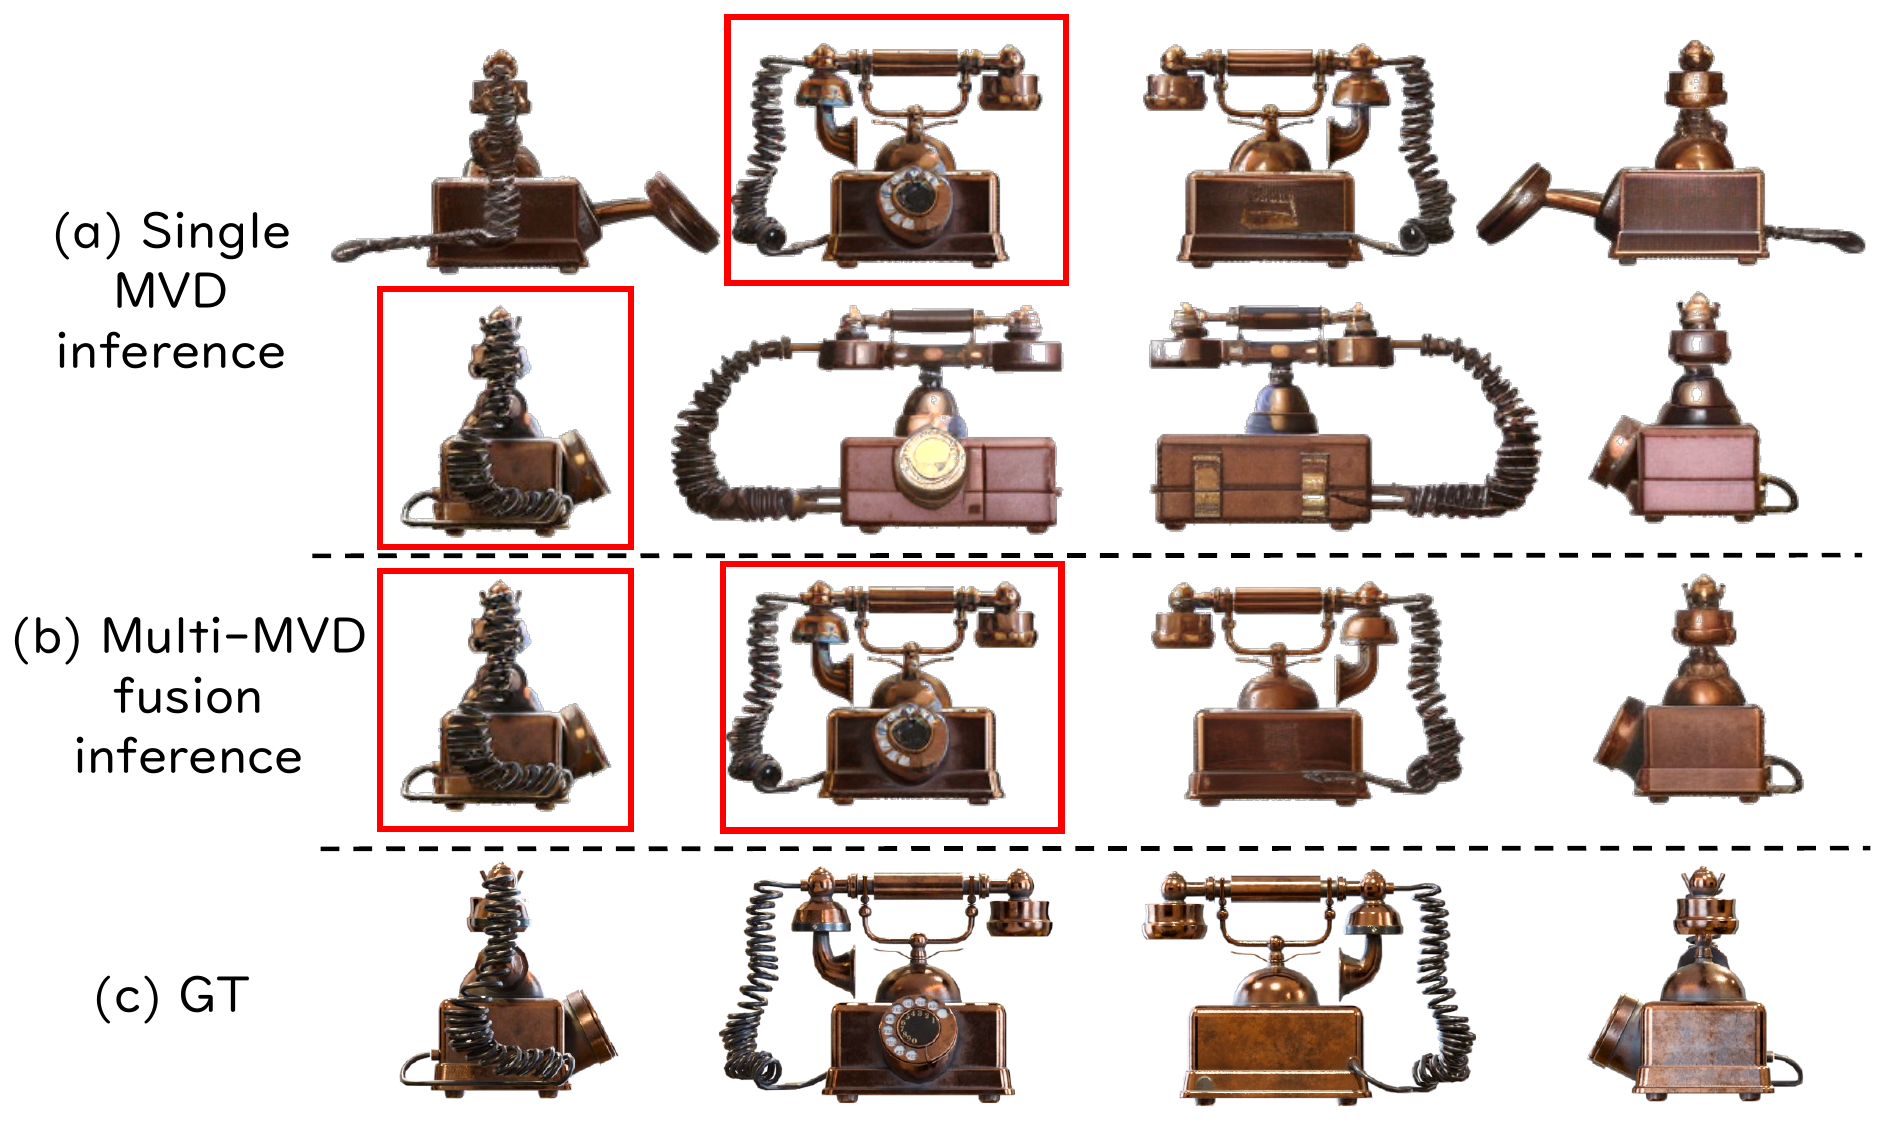}
    \caption{Generated results from multi-MVD fusion inference on Unique3D~\cite{wu2024unique3d}. As illustrated, the input images are highlighted in red boxes. The generated results utilizing multi-MVD fusion inference demonstrate remarkable fidelity to the groundtruth.}
    \label{unique3d}
    \vspace{-5}
\end{figure}
\section{Method Generalizability}
\subsection{Input Configuration Flexibility}
In scenarios where the visible regions are constrained to less than 90 degrees, our framework demonstrates adaptability by operating with two input views separated by 45 degrees for object reconstruction. As illustrated in Fig~\ref{rotation_supp_2}, although this configuration utilizes relatively limited information compared to the three-view setup, it still enables comprehensive coverage of the object's circumference. The efficacy of this approach is demonstrated through qualitative results presented in Fig.~\ref{45degree}, which showcase successful object reconstruction under such constrained viewing conditions.
\subsection{Backbone Model Compatibility}
To validate the plug-and-play compatibility of our proposed method, we conduct additional experiments using Unique3D's multi-view diffusion framework with 90-degree separated input views. The qualitative results presented in Fig.~\ref{unique3d} demonstrate that our approach significantly enhances the model's capability to capture object structure, resulting in superior reconstruction quality. This compatibility validates the generalizability of our method across different MVD architectures.
\section{Video Demonstration}
Please refer to the provided video demo, \method.mp4, for a more detailed visual comparison.
%\section{Rationale}
%\label{sec:rationale}
% 
%Having the supplementary compiled together with the main paper means that:
% 
%\begin{itemize}
%\item The supplementary can back-reference sections of the main paper, for example, we can refer to \cref{sec:intro};
%\item The main paper can forward reference sub-sections within the supplementary explicitly (e.g. referring to a particular experiment); 
%\item When submitted to arXiv, the supplementary will already included at the end of the paper.
%\end{itemize}
% 
%To split the supplementary pages from the main paper, you can use \href{https://support.apple.com/en-ca/guide/preview/prvw11793/mac#:~:text=Delete%20a%20page%20from%20a,or%20choose%20Edit%20%3E%20Delete).}{Preview (on macOS)}, \href{https://www.adobe.com/acrobat/how-to/delete-pages-from-pdf.html#:~:text=Choose%20%E2%80%9CTools%E2%80%9D%20%3E%20%E2%80%9COrganize,or%20pages%20from%20the%20file.}{Adobe Acrobat} (on all OSs), as well as \href{https://superuser.com/questions/517986/is-it-possible-to-delete-some-pages-of-a-pdf-document}{command line tools}.
